# Supplementary material for: Split-Channel Ballistic Transport in an InSb Nanowire
Source: arXiv:1709.02614 ancillary file (2018-03-09)
Supplement: Supplementary file 1 [file Estrada_et_al_SplitChannel_Sup.pdf]

# Split-Channel Ballistic Transport in an InSb Nanowire: Supplementary Information


Juan Carlos Estrada Saldaña,[†,∥] Yann-Michel Niquet,[‡] Jean-Pierre Cleuziou,[†] Eduardo J. H. Lee,[†,⊥] Diana Car,[¶] Sébastien R. Plissard,[§] Erik P. A. M. Bakkers,[¶] and Silvano De Franceschi[*,†]

†*Univ. Grenoble Alpes, INAC-PHELIQS, F-38000 Grenoble, France and CEA, INAC-PHELIQS, F-38000 Grenoble, France*

‡*Univ. Grenoble Alpes, INAC-MEM, F-38000 Grenoble, France and CEA, INAC-MEM, F-38000 Grenoble, France*

¶*Technische Universiteit Eindhoven, P.O. Box 513, 5600 MB Eindhoven*

§*CNRS, LAAS-CNRS, Université de Toulouse, 31400 Toulouse, France*

∥*Present address: Center for Quantum Devices, Niels Bohr Institute, University of Copenhagen, 2100 Copenhagen, Denmark*

⊥*Present address: Condensed Matter Physics Center (IFIMAC), Universidad Autónoma de Madrid, 28049 Madrid, Spain.*

E-mail: silvano.defranceschi@cea.fr


## dI/dV (V,$V_C$) maps: estimate of g-factors, lever-arm parameters, subband splitting

The electron g-factors and the lever-arm parameters relating variations in the central-gate voltage $V_C$ to energy variations were extracted from the stability diagrams shown in Fig.

S1, taken at B = 5 T and at different $V_G$ values. These stability diagrams were obtained by measuring the differential conductance $dI/dV$ as a function of $V_C$ and $V$, the bias voltage between source and drain contacts, using a standard lock-in technique with a bias-voltage modulation of 50 $\mu$V at 27.3 Hz. Table S1 indicates, for each value of $V_G$, the lever-arms, $\alpha_1$ and $\alpha_2$, and the g-factors, $g_1$ and $g_2$, for the first two subbands, subband 1 and 2, respectively. An estimate of the energy spacing $\Delta E$ between subband 1 and subband 2 in the limit of zero magnetic field is also provided.

Following a standard procedure, the Zeeman energy splittings and the directly related g-factors are deduced from the height of the diamonds. The lever-arm parameters are obtained from the slopes of the diamond edges. The subband splitting is deduced from the distance between the barycenters of the diamonds.

In order to estimate the uncertainty in the above mentioned parameters, we used the following procedure. We first drew by eye the best fitting line for each of the diamond edges in Fig. S1. Then we varied the position and slope of the fitting lines till they would no longer give an acceptable fit. The corresponding variations in the heights and slopes of the diamonds would then provide the experimental uncertainties on the estimated g-factors and lever-arm parameters, respectively. The error on the subband spacing is primarily related to the uncertainty in the position of the subband barycenters (black crosses).

Table S1: Estimated lever arm parameters and g-factors for the first two subbands and relative spacing ($\Delta E$)

| $V_G$ (V) | $\alpha_1$ (eV/V) | $\alpha_2$ (eV/V) | $\|g_1\|$ | $\|g_2\|$ | $\Delta E$ (meV) |
|---|---|---|---|---|---|
| 1.96 | 0.062 $\pm$ 0.010 | 0.040 $\pm$ 0.006 | 46 $\pm$ 7 | 48 $\pm$ 7 | 3 $\pm$ 2 |
| 2.5 | 0.057 $\pm$ 0.009 | 0.033 $\pm$ 0.006 | 44 $\pm$ 7 | 48 $\pm$ 9 | 11 $\pm$ 3 |
| 3.96 | 0.037 $\pm$ 0.008 | 0.029 $\pm$ 0.005 | 45 $\pm$ 9 | 44 $\pm$ 8 | 12.5 $\pm$ 3.5 |

The barycenters are located at the intersection with zero bias of the line that connects the upper and lower vertices of the diamonds. We drew all the possible diamonds that could fit the data, located their respective barycenters and drew triangles as those given by the black lines in Fig. S1 in order to convert their gate positions into bias voltage. The difference

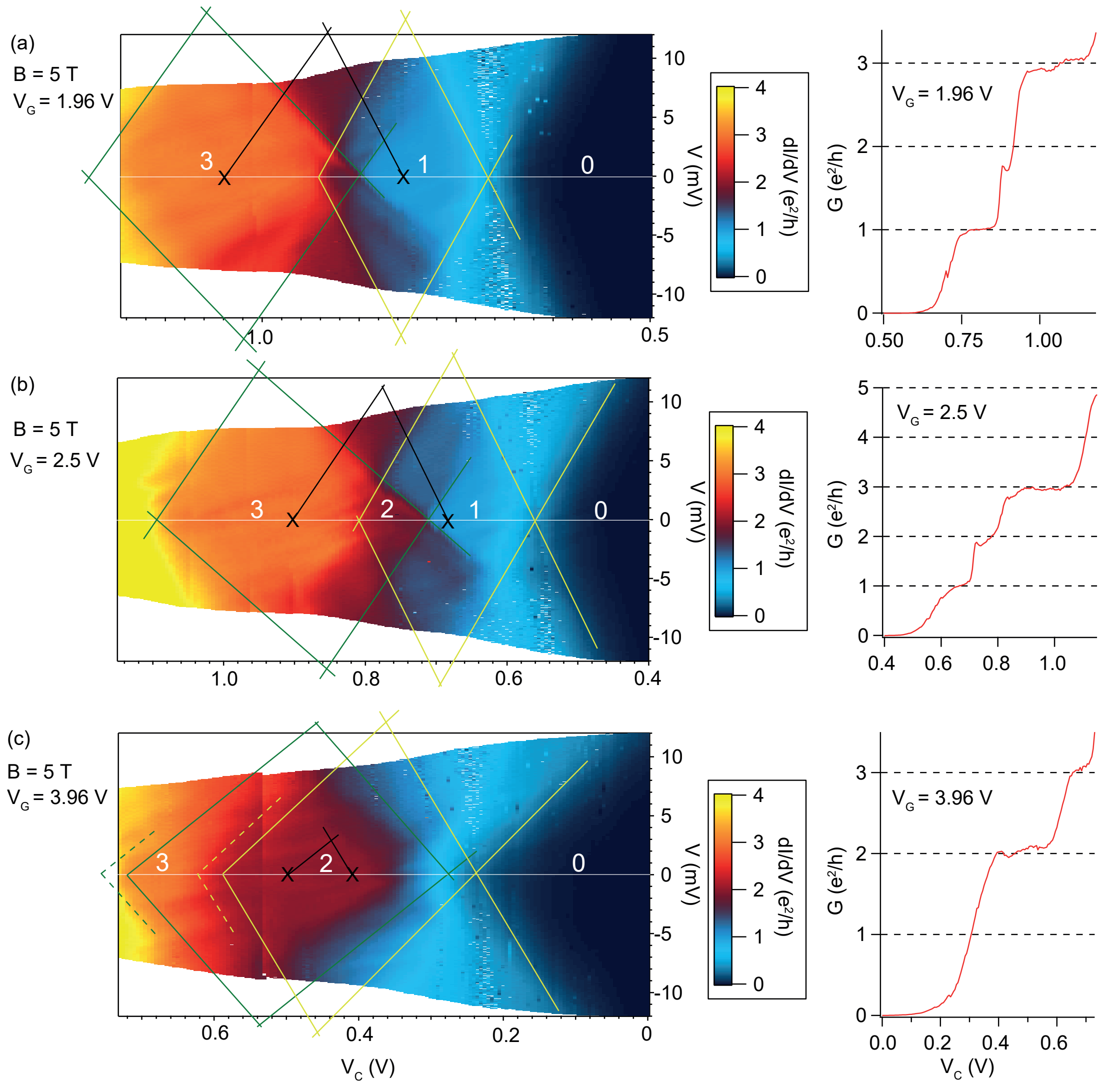


Figure S1: **Left panels:** Differential conductance $dI/dV(V_C,V)$ at $V_G = 1.96$ V (a), 2.5 V (b), and 3.96 V (c). Plateaus have been labeled by their conductance in units of $e^2/h$. Yellow (green) lines are guides for the eye to discern the diamond edges of the first (second) subband. Their slope was used to estimate the lever-arm parameter $\alpha_1$ ($\alpha_2$). Black crosses indicate the barycenters of the two subbands, i.e. their expected location at $B = 0$. The black lines are drawn parallel to the yellow and green lines in order to measure the subband spacing. In panel (c), dotted lines denote the $dI/dV$ steps observed at $V_C > 0.54$ V in the presence of a visible charge switch relative to the $V_C < 0.54$ V region. The solid lines are shifted relative to the dashed lines in order to compensate for the charge switch, reconciling the two portions of the plot and enabling a correct estimate of the lever arm parameters. **Right panels:** Corresponding line cuts at zero dc bias voltage showing the steps of quantized conductance.

in height between the smallest and the largest triangle provided the error bar in barycenter position.

The error on $\Delta E$ also contains a contribution from the uncertainty in the slope of the edges of the black triangle in Fig. S1. For the edge on the right (left) hand side, the uncertainty on the slope is proportionally the same as the one on $\alpha_1$ ($\alpha_2$).

## Resonance before the $e^2/h$ plateau

Fig. S2a shows a zoom of the G ($V_C$,$V_{G'}$) map of Fig. 4a from the main text. In this zoomed map, two resonances are seen. One appears parallel to the $2e^2/h$ plateau and was described in the main text as related to the second spin-polarized subband. The other one appears parallel to the $e^2/h$ plateau, and for this reason we associate it with the first spin-polarized subband. Interestingly, when one resonance is present, the other is absent for a fixed $V_{G'}$ voltage.

A line cut displaying this second resonance is shown in Fig. S2b. The resonance is noisy and precedes the $e^2/h$ plateau.

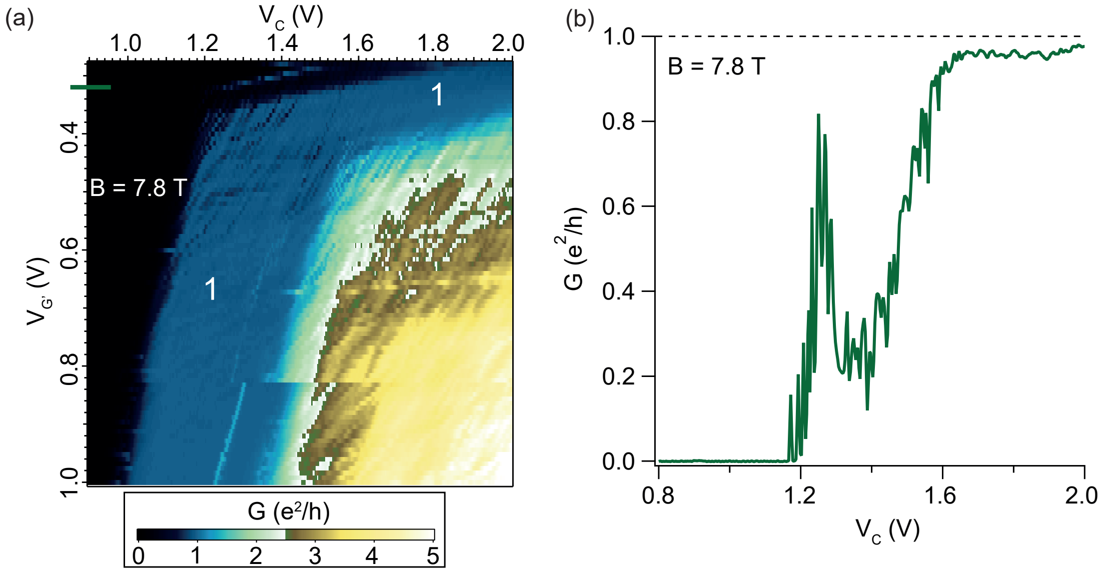


Figure S2: (a) Zoom of Fig. 4a from the main text. (b) Line cut through the map in (a) at $V_{G'} = 0.32$ V.

Due to their different capacitive coupling to the gates, it is also possible to deduce the gate above which each of these resonance forms. The resonance described in Fig. S2b is mostly affected by $V_{G'}$, while the one described in Fig. 4c of the main text is mostly affected by $V_C$.

# Subband structure of an InSb nanowire under high magnetic field

We discuss the effects of magnetic and electric fields on InSb nanowires (NWs) in the strong magnetic confinement regime, and possible scenarios for the resonances measured in the present InSb NWs.

## Simple effective mass model

At high magnetic field, the electrons get confined into cyclotron orbits. Once magnetic confinement prevails over structural confinement, these cyclotron orbits form highly degenerate 1D subbands (1D Landau levels).[S1,S2] To provide an intuitive picture of this effect, we initially consider a simple effective mass model for a NW with a square section in a magnetic field $\boldsymbol{B} = B\boldsymbol{y}$ perpendicular to the NW axis $\boldsymbol{z}$. Let $L$ be the NW lateral size.

In the Landau gauge $\boldsymbol{A} = -Bx\boldsymbol{z}$, the (spinless) effective mass Hamiltonian reads:

$$H = \frac{1}{2m^*}\left[p_x^2 + p_y^2 + (p_z - eBx)^2\right] \,, \tag{S1}$$

with boundary conditions $\psi(\pm L/2, y, z) = \psi(x, \pm L/2, z) = 0$ on the wave functions. We may factorize $\psi(x, y, z) = \varphi_{x,k}(x)\varphi_y(y)e^{ikz}$ and split the energy $E = E_{x,k} + E_y$, where $k$ is a

wave vector and:

$$-\frac{\hbar^2}{2m^*}\frac{\partial^2}{\partial x^2}\varphi_{x,k}(x)+\frac{1}{2}m^*\omega_c^2\left(x-\frac{\hbar k}{eB}\right)^2\varphi_{x,k}(x)=E_{x,k}\varphi_{x,k}(x) \tag{S2a}$$

$$-\frac{\hbar^2}{2m^*}\frac{\partial^2}{\partial y^2}\varphi_y(y)=E_y\varphi_y(y)\,, \tag{S2b}$$

with $\omega_c = eB/m^*$ the cyclotron frequency. The first equation describes a confined harmonic oscillator, whose potential reaches its minimum at $x_k = \hbar k/(eB)$. The subbands defined by this equation correspond to the different modes of the harmonic oscillator. In the limit of strong magnetic confinement $eB \gg \hbar/L^2$, these subbands are essentially flat (the energy $E_{x,k} \simeq (n+\frac{1}{2})\hbar\omega_c$ does not depend on $k$), and the corresponding $\varphi_{x,k}(x) \equiv \chi_n(x-x_k)$ are the wave functions $\chi_n$ of the harmonic oscillator, centered at $x = x_k$. In fact, the subbands acquire a finite dispersion once the harmonic oscillator wave functions start to interact with the boundaries of the wire ($x_k \to \pm L/2$). The second equation describes transverse modes with increasing number of nodes along $y$.

Therefore, in the same limit $eB \gg \hbar/L^2$ where the Landau quantization energy $\hbar\omega_c$ is significantly larger than the structural confinement energy, the lowest subbands all correspond to transverse modes along $y$. Moving along $k$ in each subband amounts to sample cyclotron orbits at different positions $x = x_k$. Note the dichotomy between the signatures of the excitations along $x$ and $y$.

## Tight-binding calculations

For a more realistic simulation, we now consider a 160-nm diameter hexagonal InSb NW in a magnetic field $B = 8$ T oriented at $\theta = 45°$ with respect to the NW axis $\boldsymbol{z} \parallel [111]$. For comparison to the experiment, we take $\boldsymbol{x}$ perpendicular to the substrate, and $\boldsymbol{y}$ parallel to the substrate plane and perpendicular to the nanowire axis. The band structure is computed with an atomistic $sp^3d^5s^*$ tight-binding model.[S3] The tight-binding method accounts for the strong non-parabolicity of the conduction band of InSb and for spin-orbit interactions, and

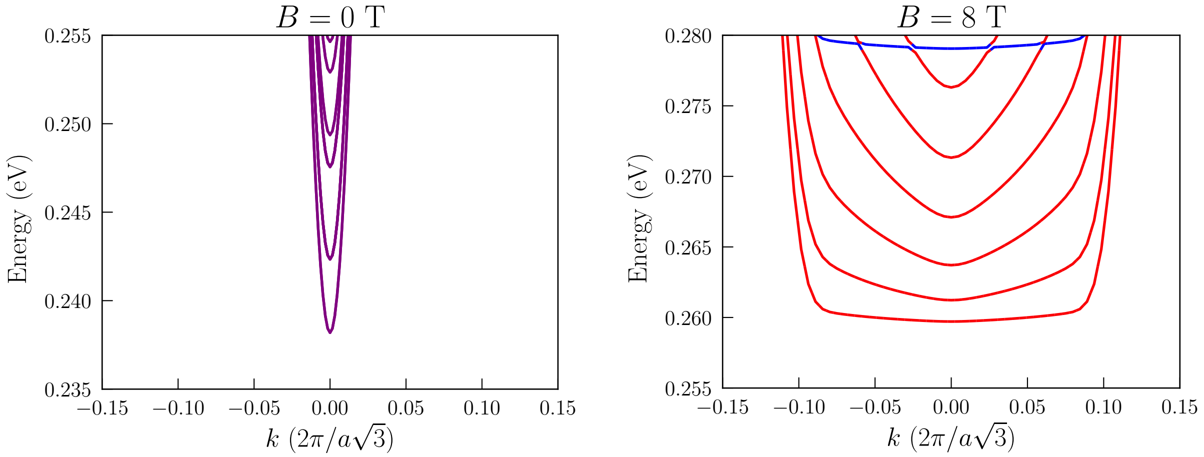


Figure S3: Band structure of a 160 nm diameter hexagonal InSb NW in a magnetic field $B = 0$ T (left) and $B = 8$ T (along $(\boldsymbol{y} + \boldsymbol{z})/\sqrt{2}$, right). $a = 6.479$ Å is the lattice parameter of InSb. Red bands are spin up bands, blue bands are spin down bands, split by the Zeeman effect. The $g$-factor of the first subband is $g = -42$.

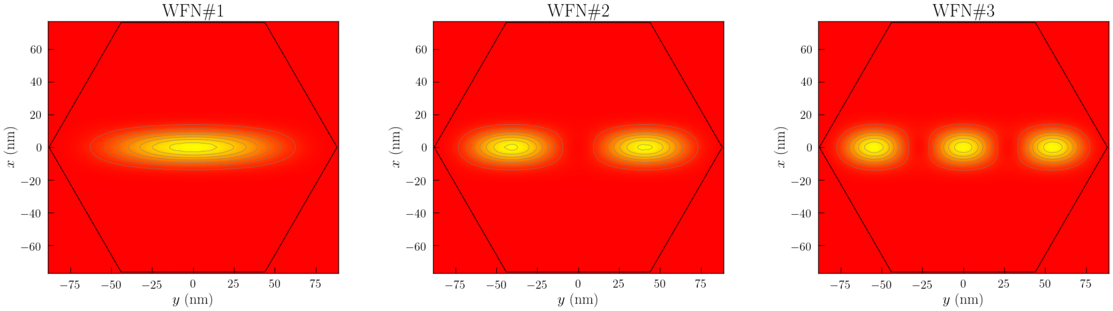


Figure S4: Squared wave functions of the first three subbands at $k = 0$ ($B = 8$ T).

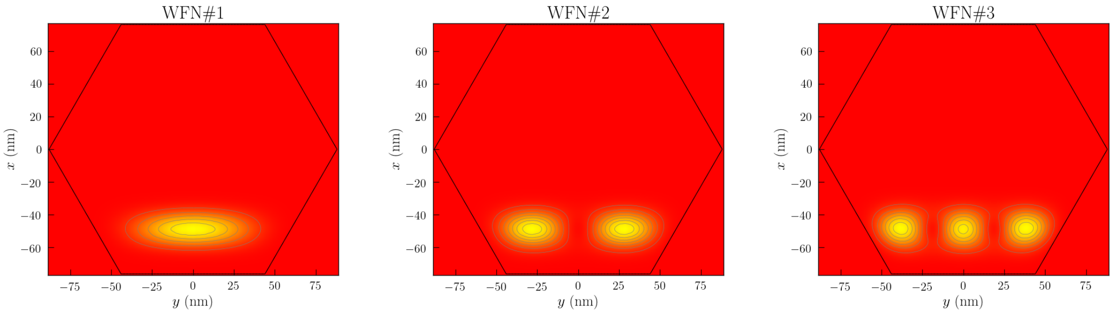


Figure S5: Squared wave functions of the first three subbands at $k = -0.075 \times 2\pi/(a\sqrt{3})$ ($B = 8$ T).

goes, therefore, far beyond the effective mass approximation. Although the magnetic field is not strictly perpendicular to the NW axis, its fingerprints remain essentially the same as in the previous section (see Fig. S3).

The lowest subbands are indeed almost flat until $x_k = \hbar k \cos\theta/(eB) \simeq \pm 60$ nm. This contrasts with the highly dispersive subbands at $B = 0$ T. The different subbands correspond to transverse modes along $y$, as illustrated by the wave functions at $k = 0$ plotted in Fig. S4. The latter are strongly confined along $x$ by the magnetic field $[(\langle x^2\rangle - \langle x\rangle^2)^{1/2} \simeq (\hbar/(2eB))^{1/2} = 6.4$ nm]. Moving along $k$ shifts the wave functions up and down along $x$, as shown in Fig. S5. This is reminiscent of the Hall effect: carriers with positive group velocity tend to accumulate on one side of the NW, while carriers with negative group velocities tend to accumulate on the other side. Note that the magnetic field can strongly limit backscattering,[S1] as the cyclotron orbits at a given Fermi energy have opposite $k$, hence opposite $x_k$. They may, therefore, little overlap, and be hardly coupled by a local disorder potential. This explains why the plateaus of conductance are more visible at high magnetic field.

## Effect of an electric field along $x$

In a "vertical" electric field $V(x) = E_x x$, the energy of a cyclotron orbit depends on $x_k$, hence on $k$ (to first-order in the electric field, $\Delta E \simeq V(x_k) \simeq E_x x_k$). Therefore, the subbands show a quasi-linear dispersion over a wide range of $k$, as illustrated in Figs. S6, S7 and S8. The subband minima are thus moved away from $k = 0$.

The dispersion of the lowest subbands does, therefore, reproduce the potential landscape along $x$ in the strong magnetic confinement regime.

Spin-orbit coupling, included in the TB calculations, is also expected to split the spin subbands in the presence of a transverse electric field.[S4,S5] This is evidenced in Fig. S6, on the close-up on the lowest conduction subbands at zero magnetic field. This structure can evolve into a helical gap at finite magnetic field. However, the characteristic energy $E_{\mathrm{SO}}$, defined as

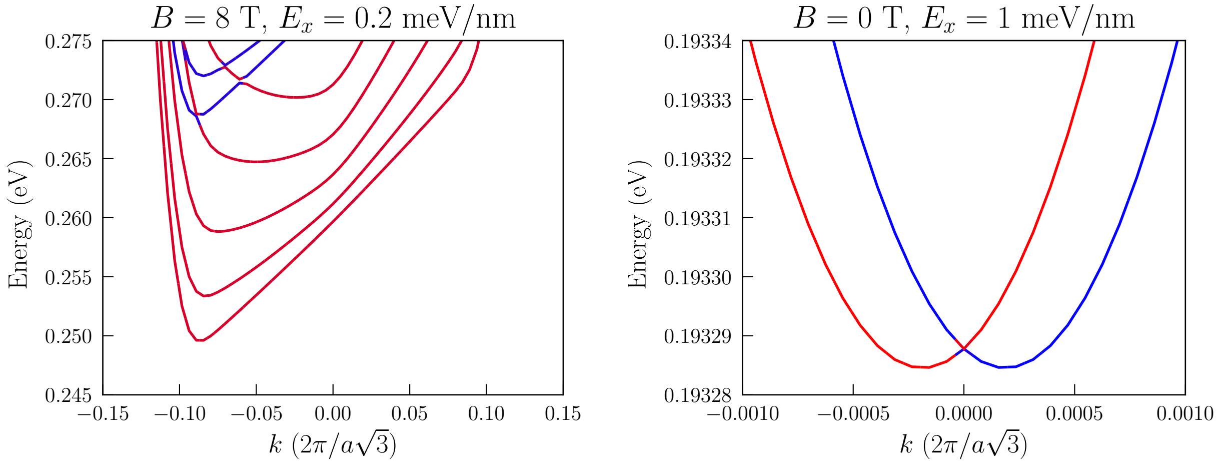


Figure S6: (left) Band structure of a 160 nm diameter hexagonal InSb NW in a magnetic field $B = 8$ T (along $(\boldsymbol{y}+\boldsymbol{z})/\sqrt{2}$), and in an electric field $E_x = 0.2$ meV/nm. (right) Band structure of 160 nm diameter hexagonal InSb NW at $B = 0$ T, in an electric field $E_x = 1$ meV/nm (close-up on the lowest subbands, showing the effects of spin-orbit coupling).

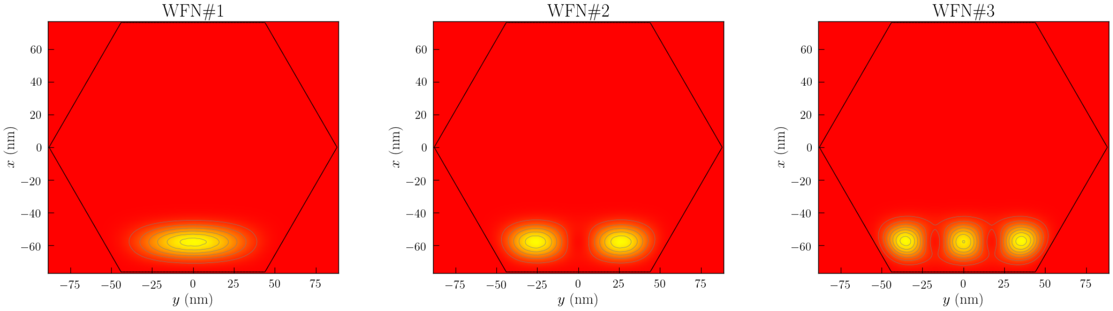


Figure S7: Squared wave functions of the first three subbands at $k = -0.089 \times 2\pi/(a\sqrt{3})$.

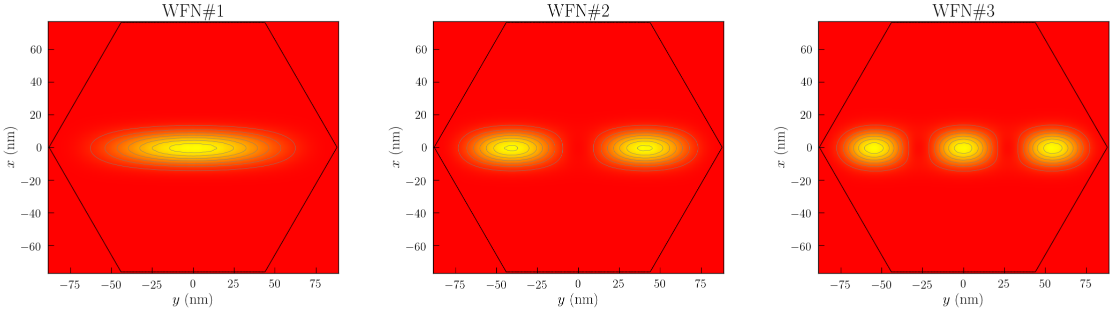


Figure S8: Squared wave functions of the first three subbands at $k = 0$.

the difference between the conduction band energy at $k = 0$ and at the edges $k = \pm k_{\rm min}$, is very small ($E_{\rm SO} \simeq 4$ $\mu$eV on Fig. S6). It hardly reaches 20 $\mu$eV for electric fields as large 10 meV/nm (which corresponds to an effective Rashba interaction $\alpha = (2\hbar^2 E_{\rm SO}/m^*)^{1/2} = 0.16$ eV.Å).[S6] Therefore, this feature is washed out at low magnetic fields by the Zeeman effect.

## Discussion

Can we explain why a resonance appears below the second subband at high enough magnetic field, and why this resonance does not seem to interact with the first subband (Breit-Wigner instead of Fano line shape) ?

First, a resonant-like structure can appear in the conductance if the potential shows two local minima along $x$, one near the top and one near the bottom of the NW (due, to, e.g., a distribution of charged surface traps). The subbands, which reproduce this potential landscape at high magnetic field (previous paragraph), then show an inverted camel back structure, with two distinct (but not necessarily equivalent) valleys at positive and negative $k$ separated by a saddle point near $k = 0$. The conductance is hence $G = e^2/h$ when the Fermi energy lies between the two minima, $G \sim 2e^2/h$ when it crosses the two valleys, and $G = e^2/h$ again when it goes above the saddle point. Note that this mechanism would give rise to the same re-entrant structure in the conductance as a helical gap, but is related to orbital instead of spin effects. Such a resonance would not, however, narrow into a thin Breit-Wigner line shape, and would appear tied to the position of the first plateau of conductance rather than to the position of the second plateau of conductance.

As discussed in the previous section, the lowest subbands correspond to transverse modes along $y$ at high magnetic field. The calculated splitting between these subbands (of the order of 2 meV at $k = 0$) is significantly smaller than the experimentally measured one. This suggests significant localization along $y$. Indeed, any modulation of the potential along $y$ with depth in the 10 meV range can easily relocalize the carriers. A resonance in the second subband may not interact with the first subband because the carriers are localized at

different $y$'s and/or different $x$'s (since the position along $x$ is directly related to the Fermi wave vectors in each subband).

As a matter of fact, even a small electric field $E_y$ of the order of 0.1 meV/nm can promote the formation of "side channels" in the NW. The effect is illustrated in the simulations of Fig. 5 in the main text. Charges with an areal density $\sigma = -2 \times 10^{12} e/cm^2$ have been introduced at the interface between InSb and $HfO_2$. These charges repel the free carriers from the bottom interface to the top, left and right of the NW. A vertical electric field $E_x = 1.9$ mV/nm has also been applied in order to mimic the vertical component of the gate-induced field. In addition, a small electric field $E_y$ from 0.1 to 0.2 mV/nm is introduced to break the symmetry between the left and right sides of the NW. $E_y$ can arise from the applied gate voltages, as the NW is not lying perpendicular to the bottom gate lines, and a possible small imbalance between the density of surface traps on the left and right of the NW.

The first and second subbands now correspond to separate left and right channels (see Fig. 5 in the main text). In this scenario, a local potential minimum along the NW axis, created by a gate-induced double-hump potential or by a charge defect, would then produce localized states either on the right or on the left side of the NW, which would couple uniquely to the subband lying on the same side. We believe this can be the nature of the resonant bound states observed in our experiment, as shown in Fig. 4 of the main text, or in Fig. S2b. This also explains the Breit-Wigner-like lineshape of the resonance in Fig. 4c.

Note that the splitting between the lowest-lying subbands has significantly increased, and that the first two subbands are spin up while the third one is spin down as in the experiment. Although the present simulation remains a "model" calculation only aimed at giving a qualitative picture of the physics of the NW, it shows that confinement by the magnetic field (along $x$) and by the potential (along $y$) can explain the experimental observations. The existence of two localized channels whose degeneracy is controlled by the gate voltages is, in particular, compatible with Figs. 2 and 4 of the main text. A more

complete analysis would require a detailed knowledge of the nature of the traps at the surface of the NW and in the high-$\kappa$ layer.

# References


[S1] Beenakker, C. W. J.; van Houten, H. In *Semiconductor Heterostructures and Nanostructures*; Ehrenreich, H., Turnbull, D., Eds.; Solid State Physics Supplement C; Academic Press, 1991; Vol. 44; pp 1–228.

[S2] Vigneau, F.; Gul, O.; Niquet, Y.-M.; Car, D.; Plissard, S. R.; Escoffier, W.; Bakkers, E. P. A. M.; Duchemin, I.; Raquet, B.; Goiran, M. Revealing the band structure of InSb nanowires by high-field magnetotransport in the quasiballistic regime. *Phys. Rev. B* **2016**, *94*, 235303.

[S3] Jancu, J.-M.; Scholz, R.; Beltram, F.; Bassani, F. Empirical spds* tight-binding calculation for cubic semiconductors: General method and material parameters. *Phys. Rev. B* **1998**, *57*, 6493–6507.

[S4] Středa, P.; Šeba, P. Antisymmetric Spin Filtering in One-Dimensional Electron Systems with Uniform Spin-Orbit Coupling. *Phys. Rev. Lett.* **2003**, *90*, 256601.

[S5] Pershin, Y. V.; Nesteroff, J. A.; Privman, V. Effect of spin-orbit interaction and in-plane magnetic field on the conductance of a quasi-one-dimensional system. *Phys. Rev. B* **2004**, *69*, 121306.

[S6] Large *homogeneous* fields can not be applied to such a NW because they close the gap. The dependence of $E_{\rm SO}$ on large electric fields was actually computed on test potentials $V(x) = V_0[1-e^{-(x-x_{\rm min})/L}]$, where $x_{\rm min}$ is the position of the base of the NW. The electric field is then $E_x = V_0/L$ at the base of the NW; it decreases exponentially within the NW so that the difference of potential between the top and bottom facets is $\Delta V = V_0$.

Here $V_0 = 0.1$ eV and $L$ is adjusted in order to match the target electric field at the base of the NW.
